# Supplementary material for: An open-source, end-to-end workflow for multidimensional photoemission spectroscopy
Source: arXiv:1909.07714 ancillary file (2020-11-14)
Supplement: Supplementary file 1 [file Xian_etal_MPESWorkflow_SI.pdf]

# Supplementary Information

# An open-source, end-to-end workflow for multidimensional photoemission spectroscopy

R. Patrick Xian[1*], Y. Acremann[2], Steinn Y. Agustsson[3], Maciej Dendzik[1], Kevin Bühlmann[2], Davide Curcio[4], Dmytro Kutnyakhov[5,6], Federico Pressacco[6], Michael Heber[5], Shuo Dong[1], Tommaso Pincelli[1], Jure Demsar[3], Wilfried Wurth[5,6,†], Philip Hofmann[4], Martin Wolf[1], Markus Scheidgen[1,7], Laurenz Rettig[1*], and Ralph Ernstorfer[1*]

[1] Fritz Haber Institute of the Max Planck Society, 14195 Berlin, Germany
[2] Laboratory for Solid State Physics, ETH Zurich, 8093 Zurich, Switzerland
[3] Department of Physics, University of Mainz, 55128 Mainz, Germany
[4] Department of Physics and Astronomy, Interdisciplinary Nanoscience Center (iNANO), Aarhus University, 8000 Aarhus C, Denmark
[5] DESY Photon Science, 22607 Hamburg, Germany
[6] Department of Physics, University of Hamburg, 22761 Hamburg, Germany
[7] Department of Physics, Humboldt University of Berlin, 12489 Berlin, Germany
[†]Deceased
*Corresponding authors: xian@fhi-berlin.mpg.de, rettig@fhi-berlin.mpg.de, ernstorfer@fhi-berlin.mpg.de

## Table of Contents

**S1 Metadata parameters and descriptions** ........ **2**
- **Supplementary Table 1** ........ 2
- **Supplementary Table 2** ........ 3
- **Supplementary Table 3** ........ 4
- **Supplementary Table 4** ........ 5

**References** ........ **5**

## S1 Metadata parameters and descriptions

Supplementary Tables 1-4 list categorized parameters currently enlisted (version 1.0) as metadata for data deposition and parsing by the experimental materials science section of the NOMAD database [1]. Each parameter contains a name, unit, description, and lineage (i.e. immediate parent in the parameter tree), as implemented in `parser-mpes` [2]. For each parameter entry, providing “None” means “not applicable to the particular experiment or quantity, unknown or undetermined during the period of experiment”.

**Supplementary Table 1: List of current general parameters.**

| Name | Unit | Description |
|---|---|---|
| experiment_location | None | Name of the city and country the experiment took place |
| experiment_date | None | Start and end dates of the experiment |
| experiment_summary | None | Descriptive summary of the content of the experiment |
| institution | None | Name of the institution hosting the facility |
| facility | None | Name of the experimental facility (e.g. in an acronym) |
| beamline | None | Name of the beamline the experiment took place |
| source_pump | None | Name or model of the pump light source |
| source_probe | None | Name or model of the probe light source |
| equipment | None | Name or model of the equipment (e.g. in an acronym) |
| sample | None | Description of the sample used in the experiment |
| measurement_axis | None | Names of the axes in measurement hardware |
| physical_axis | None | Names of the axes in physical terms |

**Supplementary Table 2: List of current source parameters**

| Name | Unit | Description |
|---|---|---|
| pump_rep_rate | Hz | Repetition rate of the pump source |
| pump_pulse_duration | fs | Pulse duration of the pump source |
| pump_wavelength | nm | Center wavelength of the pump source |
| pump_spectrum | None | Spectrum of the pump source |
| pump_photon_energy | eV | Photon energy of the pump source |
| pump_size | $mm^2$ | Full-width at half-maximum size of the pump source at or closest to the sample position |
| pump_fluence | $mJ/mm^2$ | Fluence of the pump source at or closest to the sample position |
| pump_polarization | None | Polarization of the pump source |
| pump_bunch | None | Total bunch number of the pump source |
| probe_rep_rate | Hz | Repetition rate of the probe source |
| probe_pulse_duration | fs | Pulse duration of the probe source |
| probe_wavelength | nm | Center wavelength of the probe source |
| probe_spectrum | None | Spectrum of the probe source |
| probe_photon_energy | eV | Photon energy of the probe source |
| probe_size | $mm^2$ | Full-width at half-maximum size of the probe source at or closest to the sample position |
| probe_fluence | $mJ/mm^2$ | Fluence of the probe source at or closest to the sample position |
| probe_polarization | None | Polarization of the probe source |
| probe_bunch | None | Total bunch number of the probe source |
| temporal_resolution | fs | Full-width at half-maximum of the pump-probe cross-correlation function |

**Supplementary Table 3: List of current detector parameters**

| Name | Unit | Description |
|---|---|---|
| extractor_voltage | V | Voltage between the extractor and the sample |
| work_distance | mm | Distance between the sample and the detector entrance |
| lens_names | None | Set of names for the electron-optic lenses |
| lens_voltages | V | Set of electron-optic lens voltages |
| tof_distance | m | Drift distance of the time-of-flight tube |
| tof_voltage | V | Voltage applied to the time-of-flight tube |
| sample_bias | V | Voltage bias applied to sample |
| magnification | None | Detector magnification |
| detector_voltage | V | Voltage applied to detector |
| detector_type | None | Description of the detector type (e.g. ‘MCP’, ‘CCD’, ‘CMOS’, etc.) |
| sensor_size | mm | Size of each of the imaging sensor chip on the detector |
| sensor_count | None | Number of imaging sensor chips on the detector |
| sensor_pixel_size | µm | Pixel size of the imaging sensor chip on the detector |
| x_to_momentum | $Å^{-1}$ | Pixel x axis to $k_x$ momentum calibration |
| y_to_momentum | $Å^{-1}$ | Pixel y axis to $k_y$ momentum calibration |
| tof_to_energy | eV | Time-of-flight to energy calibration |
| stage_to_delay | fs | Translation stage delay to pump-probe delay calibration |
| other_converts | None | Conversion factor between other measured and physical axes |
| momentum_resolution | $Å^{-1}$ | Momentum resolution of the detector |
| spatial_resolution | µm | Spatial resolution of the source |
| energy_resolution | eV | Energy resolution of the detector |

**Supplementary Table 4: List of current sample parameters.**

| Name | Unit | Description |
|---|---|---|
| sample_id | None | Identification number or signatures of the sample used |
| sample_state | None | Physical state of the sample (e.g. ‘gas’, ‘liquid’, ’solution’, ‘amorphous solid’, ‘vitreous solid’, ‘monocrystalline solid’, ‘polycrystalline solid’, etc.) |
| sample_purity | None | Chemical purity of the sample |
| sample_surface_term | None | Surface termination of the sample (if crystalline) |
| sample_layer | None | Sample layer or bulk structure (e.g. ‘bulk’, ‘monolayer’, ‘multilayer_2’ for bilayer, ‘multilayer_5’ for pentalayer, ‘heterostructure’, etc.) |
| sample_stacking | None | Stacking order of the solid surface (if crystalline) |
| sample_space_group | None | Space group of the sample compound (if crystalline) |
| chem_formula | None | Chemical formula of the sample |
| chem_elements | None | Symbols of the chemical elements contained in the sample |
| chem_name | None | Full chemical name of the sample |
| chem_id_cas | None | CAS registry number of the sample’s chemical content |
| sample_temp | K | Temperature of the sample at the time of measurement |
| sample_pressure | Pa | Pressure surrounding the sample at the time of measurement |
| growth_method | None | Sample growth method (e.g. ‘solution evaporation’, ‘chemical vapor transfer, ‘molecular beam epitaxy’, etc.) |
| preparation_method | None | Sample preparation method (e.g. ‘in-vacuum cleaving’, ‘ex-vacuum cleaving’, ‘ion milling’, etc.) |
| sample_vendor | None | Name of the sample vendor (e.g. a company name or ‘homemade’) |
| substrate_material | None | Material of the substrate the sample has immediate contact with |
| substrate_state | None | State of matter of the substrate material (similar options as those in the sample_state parameter) |
| substrate_vendor | None | Name of the substrate vendor (similar to options in sample_vendor) |

## References


1. Draxl, C. & Scheffler, M. NOMAD: The FAIR concept for big data-driven materials science. *MRS Bulletin* **43**, 676-682 (2018).
2. parser-mpes, https://gitlab.mpcdf.mpg.de/rpx/parser-mpes
